# Supplementary material for: Probabilistic Imputation for Time-series Classification with Missing Data
Source: arXiv:2308.06738 source file (2023-08-13)
Supplement: Supplementary file 1 [file additional.tex]

\section{Additional Experiments}
\label{app:sec:additional}
We conduct numerous ablation experiments to analyze the effect of obsdropout method. In PhysioNet2012 dataset, our models with obsdropout method outperforms at all rates. Also, in MIMIC-III datset, our technique works well on reasonable rates. Although there is much room for further analysis of effect of obsdropout on the predictive performance, these results are sufficient to show that our technique is generally effective.
